# Supplementary material for: GrappaNet: Combining Parallel Imaging with Deep Learning for Multi-Coil MRI Reconstruction
Source: arXiv:1910.12325 source file (2020-03-30)

PD 4x

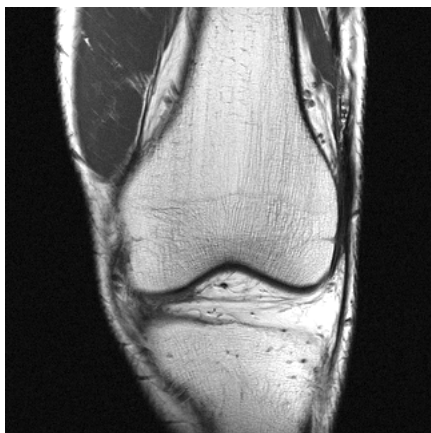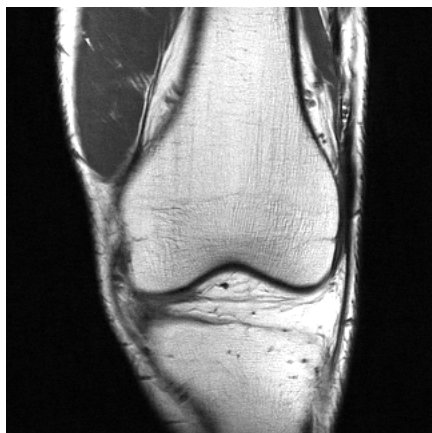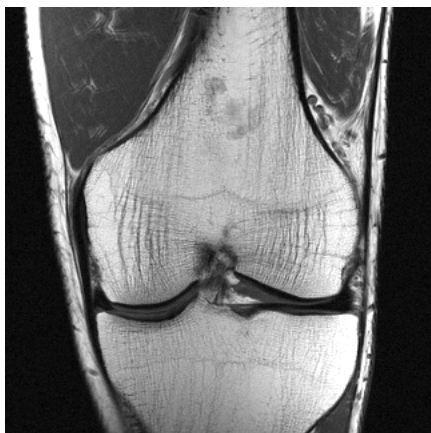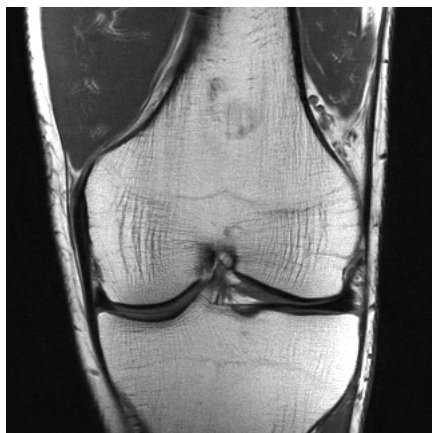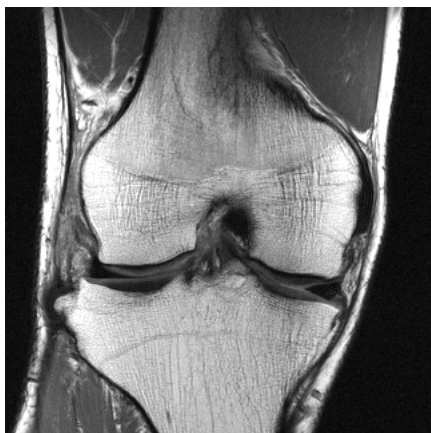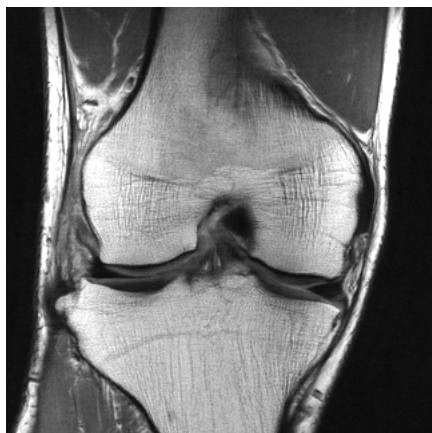

# PDFS 4x

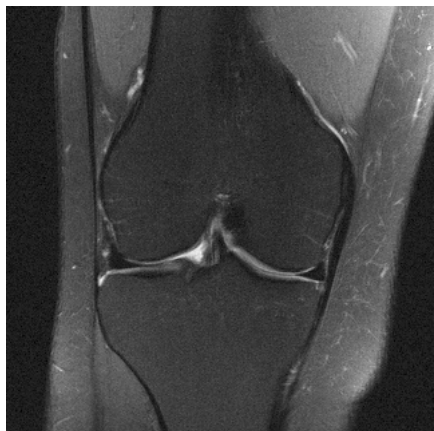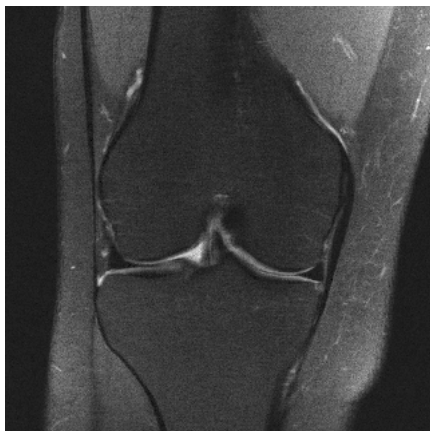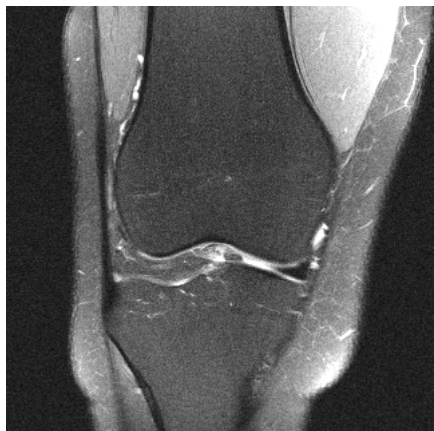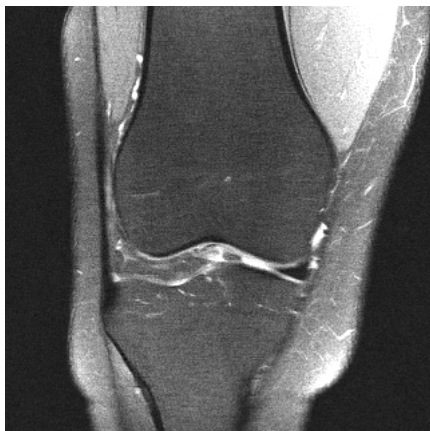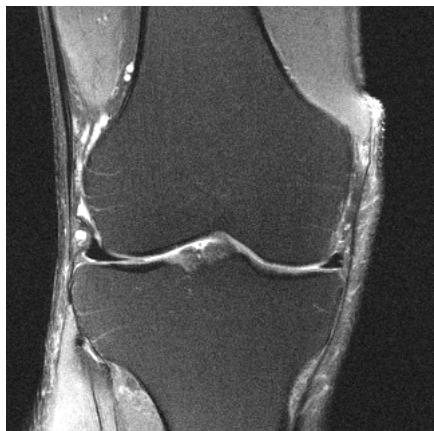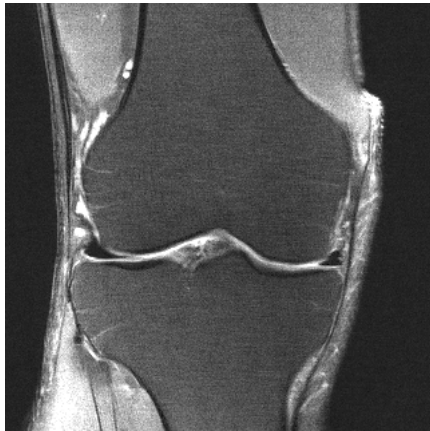

PD 8x

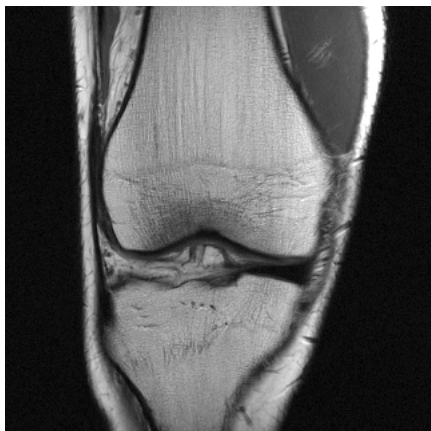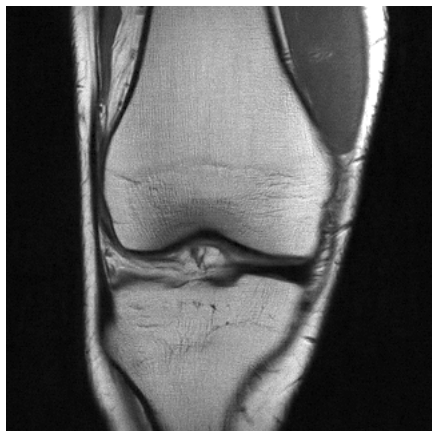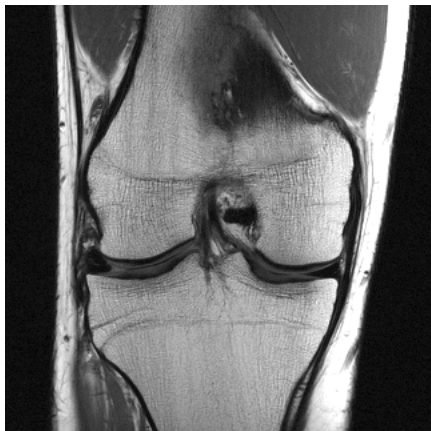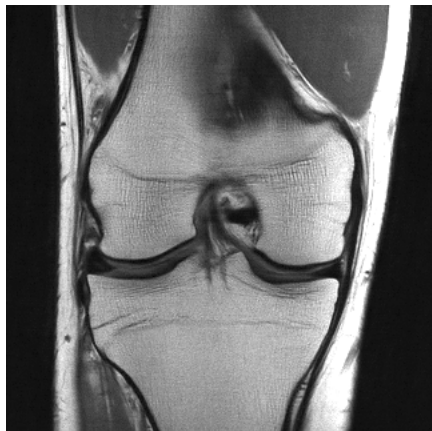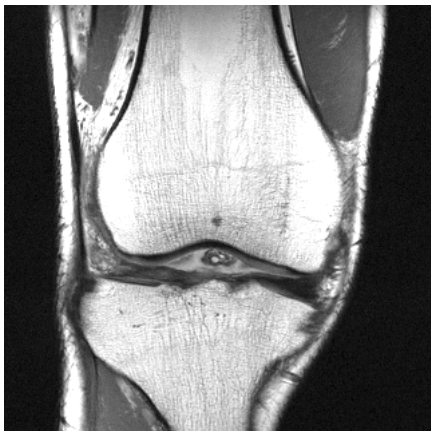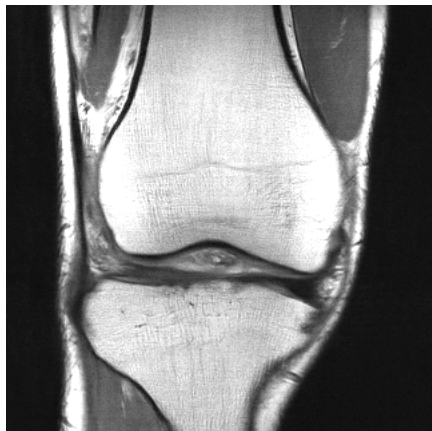

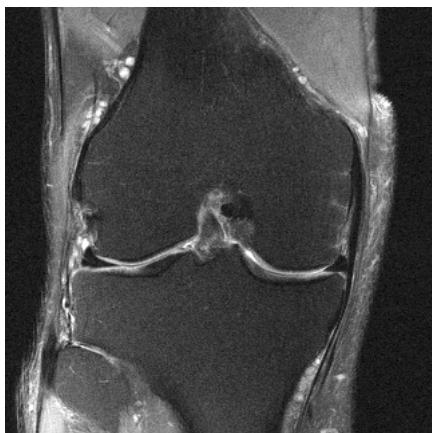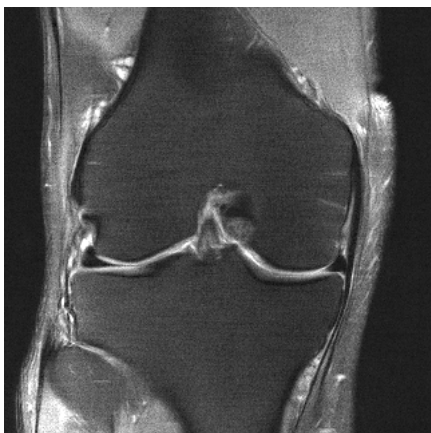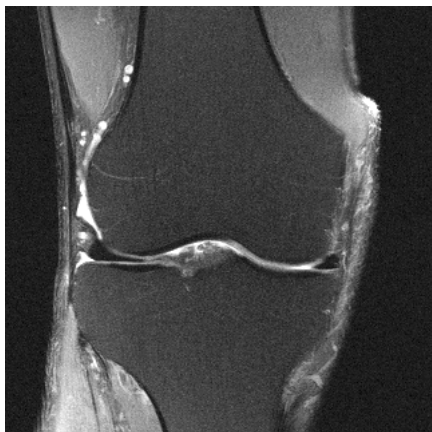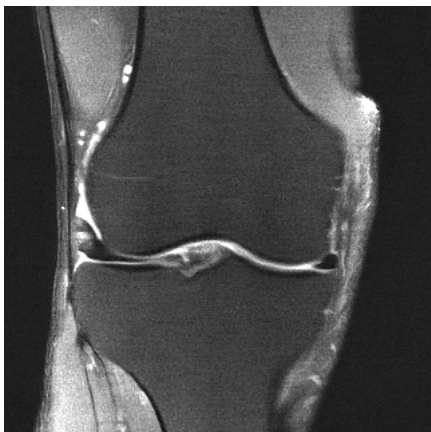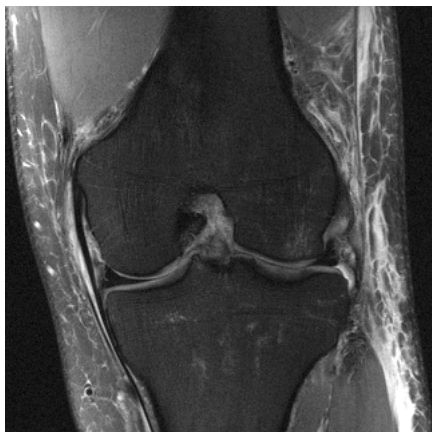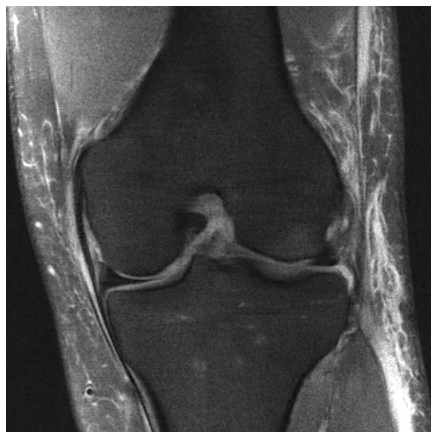

Supplement: Supplementary file 1 [file additional_images.pdf]
